# Supplementary material for: Quantum Information Engines: Assessing Time, Cost and Performance Criteria
Source: arXiv:2404.17431 source file (2024-04-26)
Supplement: Supplementary file 1 [file SM_Quantum_Information_Engines.pdf]

# Supplemental Material to
# Quantum Information Engines: Assessing Time, Cost and Performance Criteria

Henning Kirchberg* and Abraham Nitzan
*University of Pennsylvania, Department of Chemistry, Philadelphia, PA, 19104*

In Section I, the dynamics of the coupled system-meter are investigated before delving into the expectation value of the meter state in Section II. Section III examines the energy change of the meter and the measurement energy required for the measurement protocol. Section IV presents the derivation of the IE power output for the cycle time $t_m \to 0$. Finally, Section V demonstrates the maximum IE efficiency over cycle time for various operation regimes.

## I. DYNAMICS OF SYSTEM AND METER

We use an iterative numerical scheme to determine unitary time evolution of the density matrix for the coupled 2SS and meter given under the total Hamiltonian $\hat{H}$ given the initial density matrix (Eq. (2) in the main text) by

$$\begin{aligned}\hat{\rho}(t) &= e^{-i\hat{H}t/\hbar}\hat{\rho}(0)e^{i\hat{H}t/\hbar} \qquad \text{(S.1)}\\ &= a\Big(e^{-i\hat{H}_0\Delta t/\hbar}e^{-i\frac{\hat{p}^2}{2}\Delta t/\hbar}e^{-i\hat{V}\Delta t/\hbar}\Big)^N |0\rangle\langle 0| \otimes |D\rangle\langle D| \left(e^{i\hat{H}_0\Delta t/\hbar}e^{i\frac{\hat{p}^2}{2}\Delta t/\hbar}e^{i\hat{V}\Delta t/\hbar}\right)^N \\ &+ b\Big(e^{-i\hat{H}_0\Delta t/\hbar}e^{-i\frac{\hat{p}^2}{2}\Delta t/\hbar}e^{-i\hat{V}\Delta t/\hbar}\Big)^N |1\rangle\langle 1| \otimes |D\rangle\langle D| \left(e^{i\hat{H}_0\Delta t/\hbar}e^{i\frac{\hat{p}^2}{2}\Delta t/\hbar}e^{i\hat{V}\Delta t/\hbar}\right)^N,\end{aligned}$$

while using the Trotter-splitting $e^{i(\hat{H}_0+\frac{\hat{p}^2}{2}+\hat{V})t/\hbar} = \left(e^{i\hat{H}_0\Delta t/\hbar}e^{i\frac{\hat{p}^2}{2}\Delta t/\hbar}e^{i\hat{V}\Delta t/\hbar}\right)^N$ with $\Delta t = t/N$ for $N \to \infty$.

The joint probability $P_i(p,t)$ can be solved analytically using the Trotter splitting in Eq. (S.2) which results to

$$\begin{aligned}P_i(p,t) &= \sum_i \langle i|\langle p|\hat{\rho}(t)|p\rangle|i\rangle = \sum_i \langle i|\langle p| e^{-i\hat{H}t/\hbar}\hat{\rho}(0)e^{i\hat{H}t/\hbar}|p\rangle|i\rangle \qquad \text{(S.2)}\\ &= a\langle D|\langle 0|\left(e^{i\hat{H}_0\Delta t/\hbar}e^{i\frac{\hat{p}^2}{2}\Delta t/\hbar}e^{i\hat{V}\Delta t/\hbar}\right)^N|0\rangle\langle 0| \\ &\otimes |p\rangle\langle p|\left(e^{-i\hat{H}_0\Delta t/\hbar}e^{-i\frac{\hat{p}^2}{2}\Delta t/\hbar}e^{-i\hat{V}\Delta t/\hbar}\right)^N|0\rangle|D\rangle \\ &+ b\langle D|\langle 1|\left(e^{i\hat{H}_0\Delta t/\hbar}e^{i\frac{\hat{p}^2}{2}\Delta t/\hbar}e^{i\hat{V}\Delta t/\hbar}\right)^N|1\rangle\langle 1| \\ &\otimes |p\rangle\langle p|\left(e^{-i\hat{H}_0\Delta t/\hbar}e^{-i\frac{\hat{p}^2}{2}\Delta t/\hbar}e^{-i\hat{V}\Delta t/\hbar}\right)^N|1\rangle|D\rangle \\ &= a|\langle p|D\rangle|^2 \\ &+ b\int ds\int dm\int ds'\int dm'\int dx\,\langle D(s)|s\rangle\, e^{i\frac{s^2}{2}\Delta t/\hbar}\langle s|x\rangle\, e^{igx\Delta t/\hbar}\langle x|m\rangle \qquad \text{(S.3)}\\ &\langle m|\left(e^{i\frac{\hat{p}^2}{2}\Delta t/\hbar}e^{ig\hat{x}\Delta t/\hbar}\right)^{N-1}|p\rangle\langle p|\left(e^{-i\frac{\hat{p}^2}{2}\Delta t/\hbar}e^{-ig\hat{x}\Delta t/\hbar}\right)^{N-1}|m'\rangle \\ &\langle m'|e^{-i\frac{\hat{p}^2}{2}\Delta t/\hbar}|s'\rangle\langle s'|e^{-ig\hat{x}\Delta t/\hbar}|D\rangle \\ &= a|\langle p|D\rangle|^2 \\ &+ b\langle D|p+gN\Delta t\rangle\,\Pi_{k=1}^N\left[e^{i(p+gk\Delta t)^2\Delta t/2\hbar}\right] \qquad \text{(S.4)}\\ &\Pi_{k=1}^N\left[e^{-i(p+gk\Delta t)^2\Delta t/2\hbar}\right]\langle p+gN\Delta t|D\rangle \\ &= a|D(p)|^2 + b|D(p+gN\Delta t)|^2 = a|D(p)|^2 + b|D(p+gt)|^2,\end{aligned}$$

where we have exploit the completeness relation for the momentum eigenstates $\int dm\,|m\rangle\langle m| = \int dm'\,|m'\rangle\langle m'| = \int ds\,|s\rangle\langle s| = \int ds'\,|s'\rangle\langle s'| = \mathbb{I}$ and for the position eigenstates $\int dx\,|x\rangle\langle x| = \mathbb{I}$ in line (S.3). Using the relation $\langle x|m\rangle = e^{imxt/\hbar}/\sqrt{2\pi}$ and the identity $\int dx e^{i(q-a)x/\hbar} = 2\pi\delta(q-a)$, one arrives iteratively to the expression in line (S.4).

* khenning@sas.upenn.edu

## II. AVERAGE METER STATE

The expectation value of the meter outcome $\langle p(t_m)\rangle$ after the measurement of duration $t_m$, while using the Trotter-splitting $e^{i(\hat{H}_0+\frac{\hat{p}^2}{2}+\hat{V})t_m/\hbar} = \left(e^{i\hat{H}_0\Delta t/\hbar}e^{i\frac{\hat{p}^2}{2}\Delta t/\hbar}e^{i\hat{V}\Delta t/\hbar}\right)^N$ with $\Delta t = t_m/N$ for $N\to\infty$, reads

$$\begin{aligned}
\langle p(t_m)\rangle &= \mathrm{tr}[\hat{\rho}(t_m)\hat{p}] \\
&= a\,\langle D|\,\langle 0|\left(e^{i\hat{H}_0\Delta t/\hbar}e^{i\frac{\hat{p}^2}{2}\Delta t/\hbar}e^{i\hat{V}\Delta t/\hbar}\right)^N\hat{p}\left(e^{-i\hat{H}_0\Delta t/\hbar}e^{-i\frac{\hat{p}^2}{2}\Delta t/\hbar}e^{-i\hat{V}\Delta t/\hbar}\right)^N|0\rangle\,|D\rangle \\
&+ b\,\langle D|\,\langle 1|\left(e^{i\hat{H}_0\Delta t/\hbar}e^{i\frac{\hat{p}^2}{2}\Delta t/\hbar}e^{i\hat{V}\Delta t/\hbar}\right)^N\hat{p}\left(e^{-i\hat{H}_0\Delta t/\hbar}e^{-i\frac{\hat{p}^2}{2}\Delta t/\hbar}e^{-i\hat{V}\Delta t/\hbar}\right)^N|1\rangle\,|D\rangle \\
&= bg\int_{-\infty}^{\infty} dpD(p+gN\Delta t)\Pi_{k=1}^N\left[e^{i(p+gk\Delta t)^2\Delta t/2\hbar}\right]p\Pi_{k=1}^N\left[e^{-i(p+gk\Delta t)^2\Delta t/2\hbar}\right]D(p+gN\Delta t) \\
&= bg\left(\frac{2}{\pi\hbar^2 B}\right)^{1/2}\int_{-\infty}^{\infty} dpe^{-2(p+gt_m)^2/\hbar^2 B}p = -bgt_m.
\end{aligned} \tag{S.5}$$

## III. ENERGY TRANSFER DURING MEASUREMENT

We determine now the expected energy of the system, meter and their mutual coupling after (unitary) time evolution $t_m$. We consider first the average energy change of the meter (change of kinetic energy of the free particle) $\langle \Delta W_M(t_m)\rangle = \frac{1}{2}(\langle \hat{p}^2(t_m)\rangle - \langle \hat{p}^2(0)\rangle)$ after the entangling system-meter evolution of time $t_m$ by using the Trotter splitting as in Eq. (S.5) with $\Delta t = t_m/N$

$$\begin{aligned}
W_M(t_m) &= \frac{1}{2}\left[\mathrm{tr}[\hat{\rho}(t_m)\hat{p}^2] - \mathrm{tr}[\hat{\rho}(0)\hat{p}^2]\right] \\
&= \frac{b}{2}\Big[\langle D|\left(e^{i\hat{p}^2\Delta t/2\hbar}e^{i\hat{V}\Delta t/\hbar}\right)^N\hat{p}^2\left(e^{-i\hat{p}^2\Delta t/2\hbar}e^{-i\hat{V}\Delta t/\hbar}\right)^N|D\rangle \\
&- \langle D|\,\hat{p}^2\,|D\rangle\Big] \\
&= \frac{b}{2}\left(\frac{2}{\pi\hbar^2 B}\right)^{1/2}\left[\int_{-\infty}^{\infty} dpe^{-\frac{2(p+gN\Delta t)^2}{\hbar^2 B}}p^2 - \int_{-\infty}^{\infty} dpe^{-\frac{2p^2}{\hbar^2 B}}p^2\right] \\
&= \frac{bg^2 t_m^2}{2}.
\end{aligned} \tag{S.6}$$

Note that the $\langle \delta\hat{p}^2(t_m)\rangle = \langle \hat{p}^2(t_m)\rangle - \langle p(t_m)\rangle^2 \equiv 2\langle \Delta W_M(t_m)\rangle$. Consider next the change in expectation value of the system-meter coupling during evolution of time $t_m$ by using the Trotter splitting as in Eq. (S.5) with $\Delta t = t_m/N$ and

where $\hat{V} = g\hat{x} \otimes |1\rangle\langle 1|$,

$$\begin{aligned}
W_{meas}(t_m) &= -\Big[\mathrm{tr}[\hat{\rho}(t_m)\hat{V}] - \mathrm{tr}[\hat{\rho}(0)\hat{V}]\Big] \qquad \text{(S.7)}\\
&= -bg\,\langle D|\left(e^{i\hat{p}^2\Delta t/2\hbar}e^{i\hat{V}\Delta t/\hbar}\right)^N \hat{x}\left(e^{-i\hat{p}^2\Delta t/2\hbar}e^{-i\hat{V}\Delta t/\hbar}\right)^N |D\rangle\\
&= -bg\left(\frac{2}{\pi\hbar^2 B}\right)^{1/2}\Big[\int_{-\infty}^{\infty} dp e^{-\frac{(p+gN\Delta t)^2}{\hbar^2 B}} \prod_{k=1}^{N}\Big[e^{i(p+gk\Delta t)^2\Delta t/2\hbar}\Big] i\hbar\frac{d}{dp}\\
&\Big\{\prod_{k=1}^{N}\Big[e^{-i(p+gk\Delta t)^2\Delta t/2\hbar}\Big]e^{-\frac{(p+gN\Delta t)^2}{\hbar^2 B}}\Big\}\Big]\\
&= -bg\left(\frac{2}{\pi\hbar^2 B}\right)^{1/2}\Big[\int_{-\infty}^{\infty} dp e^{-\frac{2(p+gN\Delta t)^2}{\hbar^2 B}} \sum_{k=1}^{N}(p+gk\Delta t)\Delta t/\Big]\\
&= -bg\left(\frac{2}{\pi\hbar^2 B}\right)^{1/2}\Big[\int_{-\infty}^{\infty} dp e^{-\frac{2(p+gN\Delta t)^2}{\hbar^2 B}} \big(pN\Delta t + \sum_{k=1}^{N} gk\Delta t^2\big)\Big]\\
&= -bg\left(\frac{2}{\pi\hbar^2 B}\right)^{1/2}\Big[\int_{-\infty}^{\infty} dp e^{-\frac{2(p+gN\Delta t)^2}{\hbar^2 B}} \big(pt_m + gN(N+1)(t_m/N)^2/2\big)\Big]\\
&= -bg\Big[\big(-gt_m^2/M + gt_m^2/2 + gt_m^2/2N\big)\Big]\\
&\underset{\lim N\to\infty}{=} \frac{bg^2t_m^2}{2}.
\end{aligned}$$

As expected from unitary evolution, $W_M(t_m) = W_{meas}(t_m)$.

## IV. POWER FOR $t_m \to 0$

We now determine the Power $\Pi(t_m, p')$ (Eq. (12) in the main text) in the limit $t_m \to 0$.

$$\begin{aligned}
\Pi(t_m,p') &= \frac{W_{out}(t_m,p')}{t_m} = \frac{\Delta E \int_{-\infty}^{p'} dpQ(p,t_m)[P_1(t_m|p) - P_1(0|p)]}{t_m} \qquad \text{(S.8)}\\
&= \sqrt{\frac{2}{\pi}}\frac{ab\Delta E\big[\int_{-\infty}^{p'+gt_m} dpe^{\frac{-p^2}{\hbar^2 B}} - \int_{-\infty}^{p'} dpe^{\frac{-p^2}{\hbar^2 B}}\big]}{t_m} = \sqrt{\frac{2}{\pi}}\frac{ab\Delta E\big[\int_{-\infty}^{(p'+gt_m)/\hbar\sqrt{B}} e^{\frac{-p^2}{\hbar^2 B}} - \int_{-\infty}^{p'/\hbar\sqrt{B}} e^{\frac{-p^2}{\hbar^2 B}}\big]}{t_m}\\
\lim_{t_m\to 0} &= \sqrt{\frac{2}{\pi}}ab\Delta E e^{\frac{-p'^2}{\hbar^2 B}}.
\end{aligned}$$

## V. MAXIMUM EFFICIENCY FOR DIFFERENT INITIAL THERMAL STATE

Fig. S.1 shows the efficiency $\eta_{max} \equiv \eta(t_m, p'_{max})$ against the measurement time $t_m$ for different IE model parameter. The green curve corresponds to regimes of $W_{out} > W_{in}$ as discussed in the main text.

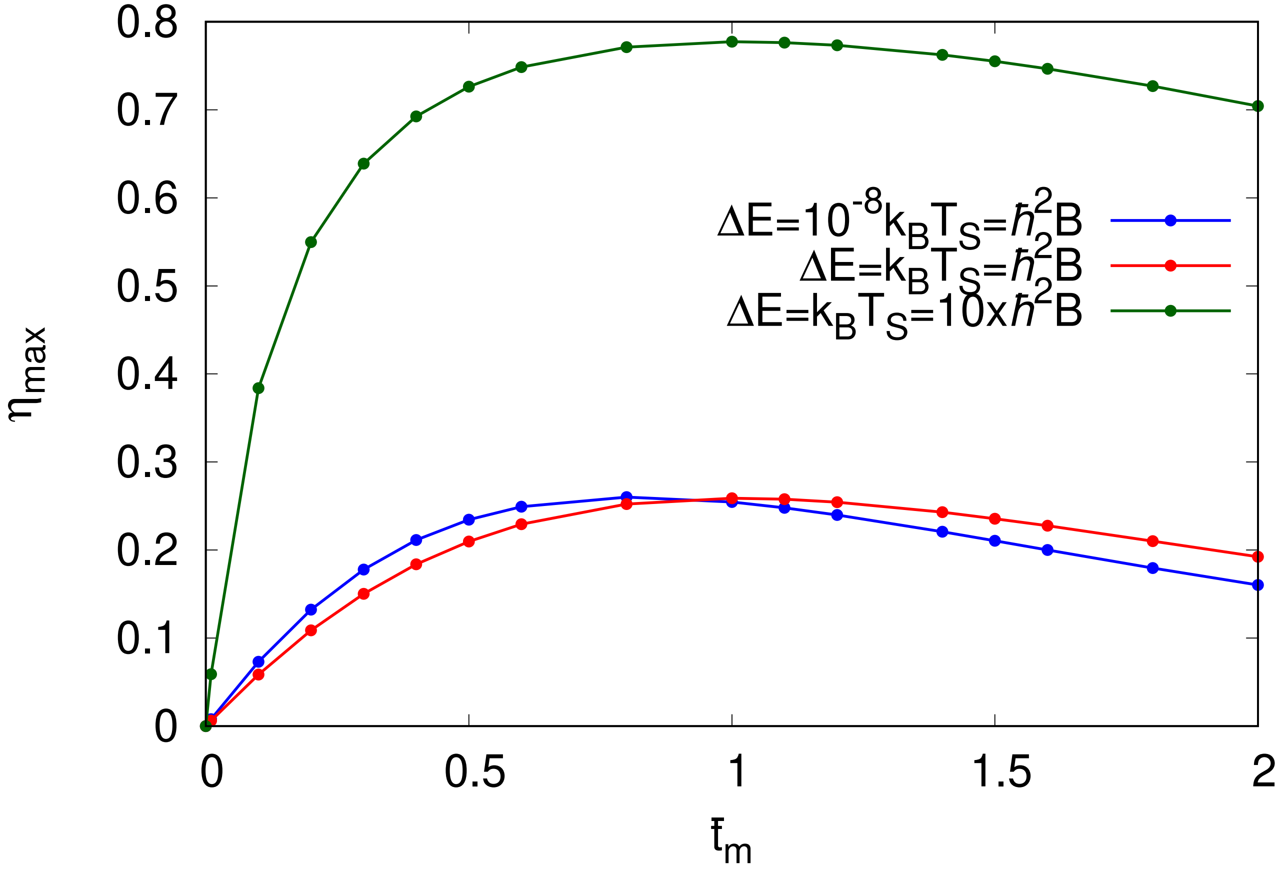


FIG. S.1. Maximal efficiency $\eta_{max}(t_m, p'_{max})$ (Eq. (11) in the main text) at outcome $p'_{max}$ as function of system-meter interaction time $t_m$ for different initial state of the 2SS defined by the temperature $a/b = e^{\Delta E/k_B T_S}$ where we choose $\Delta E = 25.58$meV (which corresponds to $k_B T$ for 300K).
